# Supplementary material for: Think Locally, Act Globally: Federated Learning with Local and Global Representations
Source: arXiv:2001.01523 source file (2020-07-14)
Supplement: Supplementary file 1 [file maps_supp.tex]

\definecolor{gg}{RGB}{15,125,15}
\definecolor{rr}{RGB}{190,45,45}

\begin{table*}[!tbp]
\fontsize{8.5}{11}\selectfont
\centering
\caption{Extra results on MAPS dataset.}
\setlength\tabcolsep{1.0pt}

\begin{tabular}{l l || c c c c c}
\Xhline{3\arrayrulewidth}
Data & \multirow{1}{*}{Method} &  \multirow{1}{*}{Local Test Acc. $(\uparrow)$} & \multirow{1}{*}{Params Comm. $(\downarrow)$} \\
\Xhline{0.5\arrayrulewidth}
\multirow{3}{*}{\rotatebox{90}{MAPS}} & \fed~\citep{DBLP:journals/corr/McMahanMRA16} & \\
& Local only~\citep{DBLP:journals/corr/SmithCST17} & \\
& \ours\ (ours) & \\
%\Xhline{0.5\arrayrulewidth}
\Xhline{3\arrayrulewidth}
\end{tabular}

\label{maps_supp}
\vspace{-4mm}
\end{table*}
